# Supplementary material for: One-Step Image Translation with Text-to-Image Models
Source: arXiv:2403.12036 source file (2024-03-18)
Supplement: Supplementary file 1 [file supplement.tex]

\documentclass[runningheads]{llncs}

\usepackage[review,year=2024,ID=2946]{eccv}

\input{macros/preamble}
\input{macros/common}
\input{macros/paper_specific}
\input{macros/authors}

\usepackage{eccvabbrv}

\usepackage[accsupp]{axessibility}  %

\usepackage[pagebackref,breaklinks,colorlinks,citecolor=eccvblue]{hyperref}

\usepackage{orcidlink}

\begin{document}

\title{Supplement: One-Step Image Translation \\ with Text-to-Image Models
\vspace{-0.1in}}
\titlerunning{CycleGAN-Turbo}

\maketitle

\input{figures/tex_supp/updated_teaser}
\input{sections/supplement/s0_overview}

\input{sections/supplement/s1_additional_ablations}
\input{sections/supplement/s2_baseline_cmp}
\input{sections/supplement/s3_additional_analysis}

\input{sections/supplement/s4_training_details}

\clearpage
{\small
\bibliographystyle{splncs04}
\bibliography{main}
}
\end{document}
